# Supplementary material for: Photon Limited Non-Blind Deblurring Using Algorithm Unrolling
Source: arXiv:2110.15314 source file (2022-10-27)
Supplement: Supplementary file 1 [file Supplemenatry.pdf]

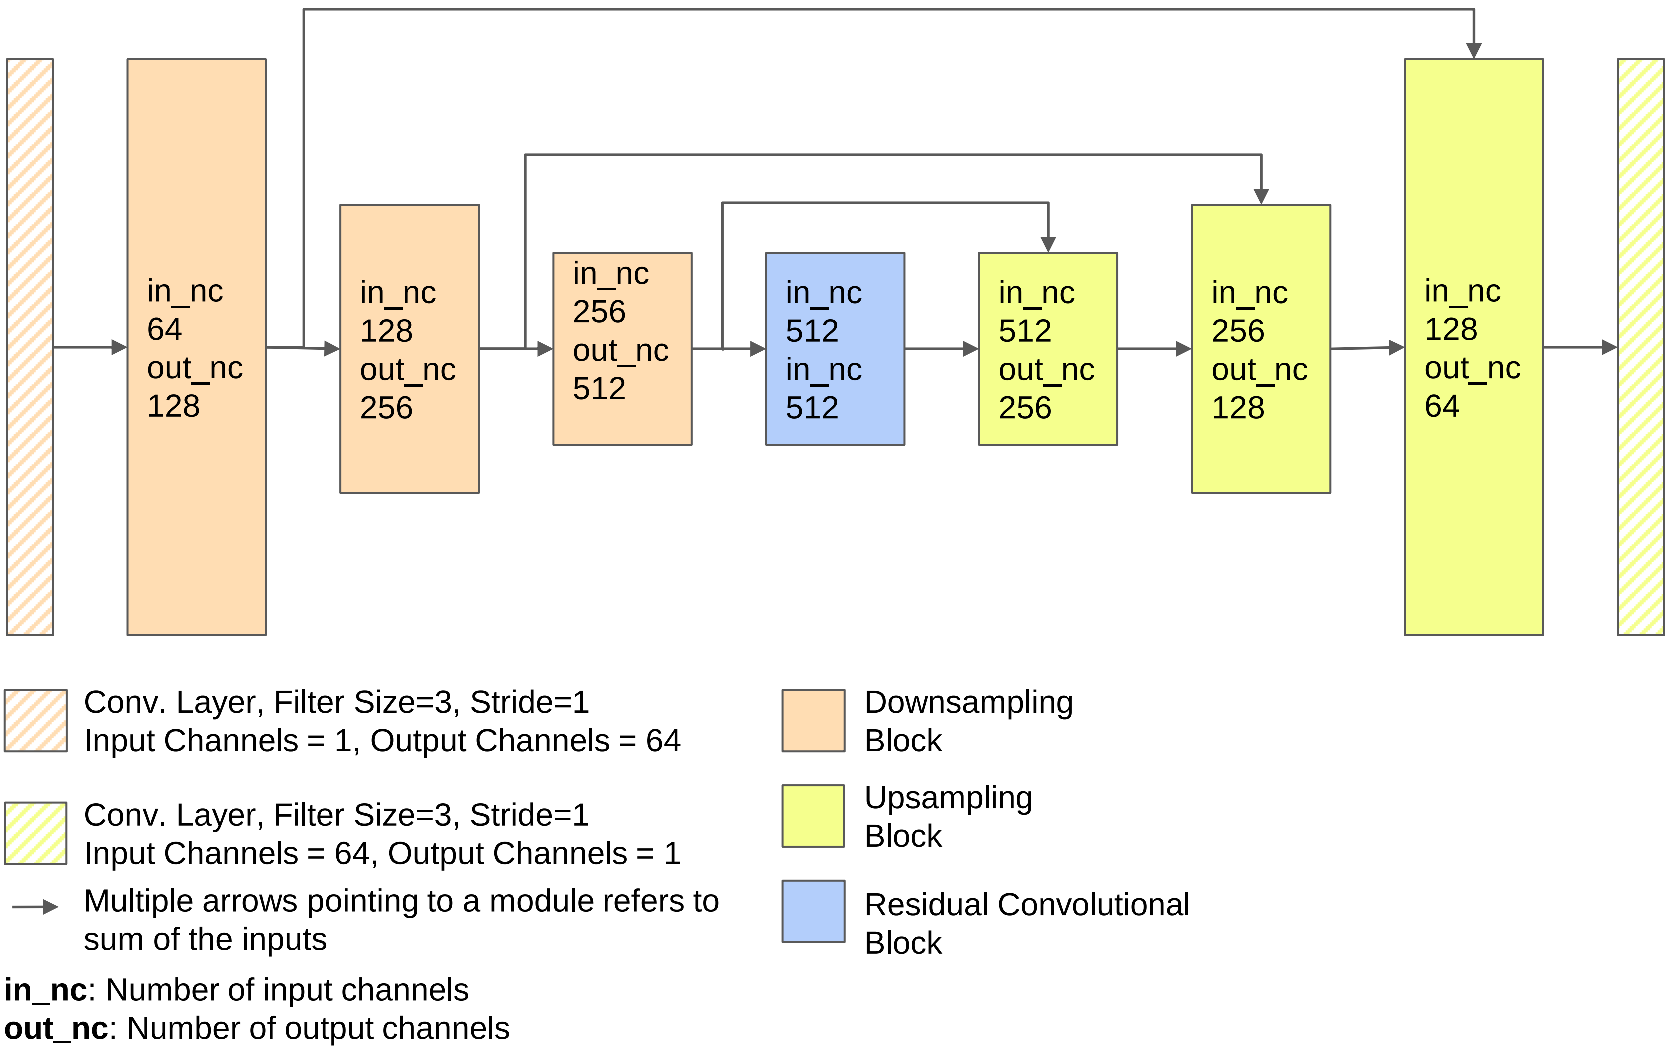

in_nc 64 out_nc 128
in_nc 128 out_nc 256
in_nc 256 out_nc 512
in_nc 512 in_nc 512
in_nc 512 out_nc 256
in_nc 256 out_nc 128
in_nc 128 out_nc 64
Conv. Layer, Filter Size=3, Stride=1
Input Channels = 1, Output Channels = 64
Conv. Layer, Filter Size=3, Stride=1
Input Channels = 64, Output Channels = 1
Multiple arrows pointing to a module refers to sum of the inputs
in_nc: Number of input channels
out_nc: Number of output channels
Downsampling Block
Upsampling Block
Residual Convolutional Block

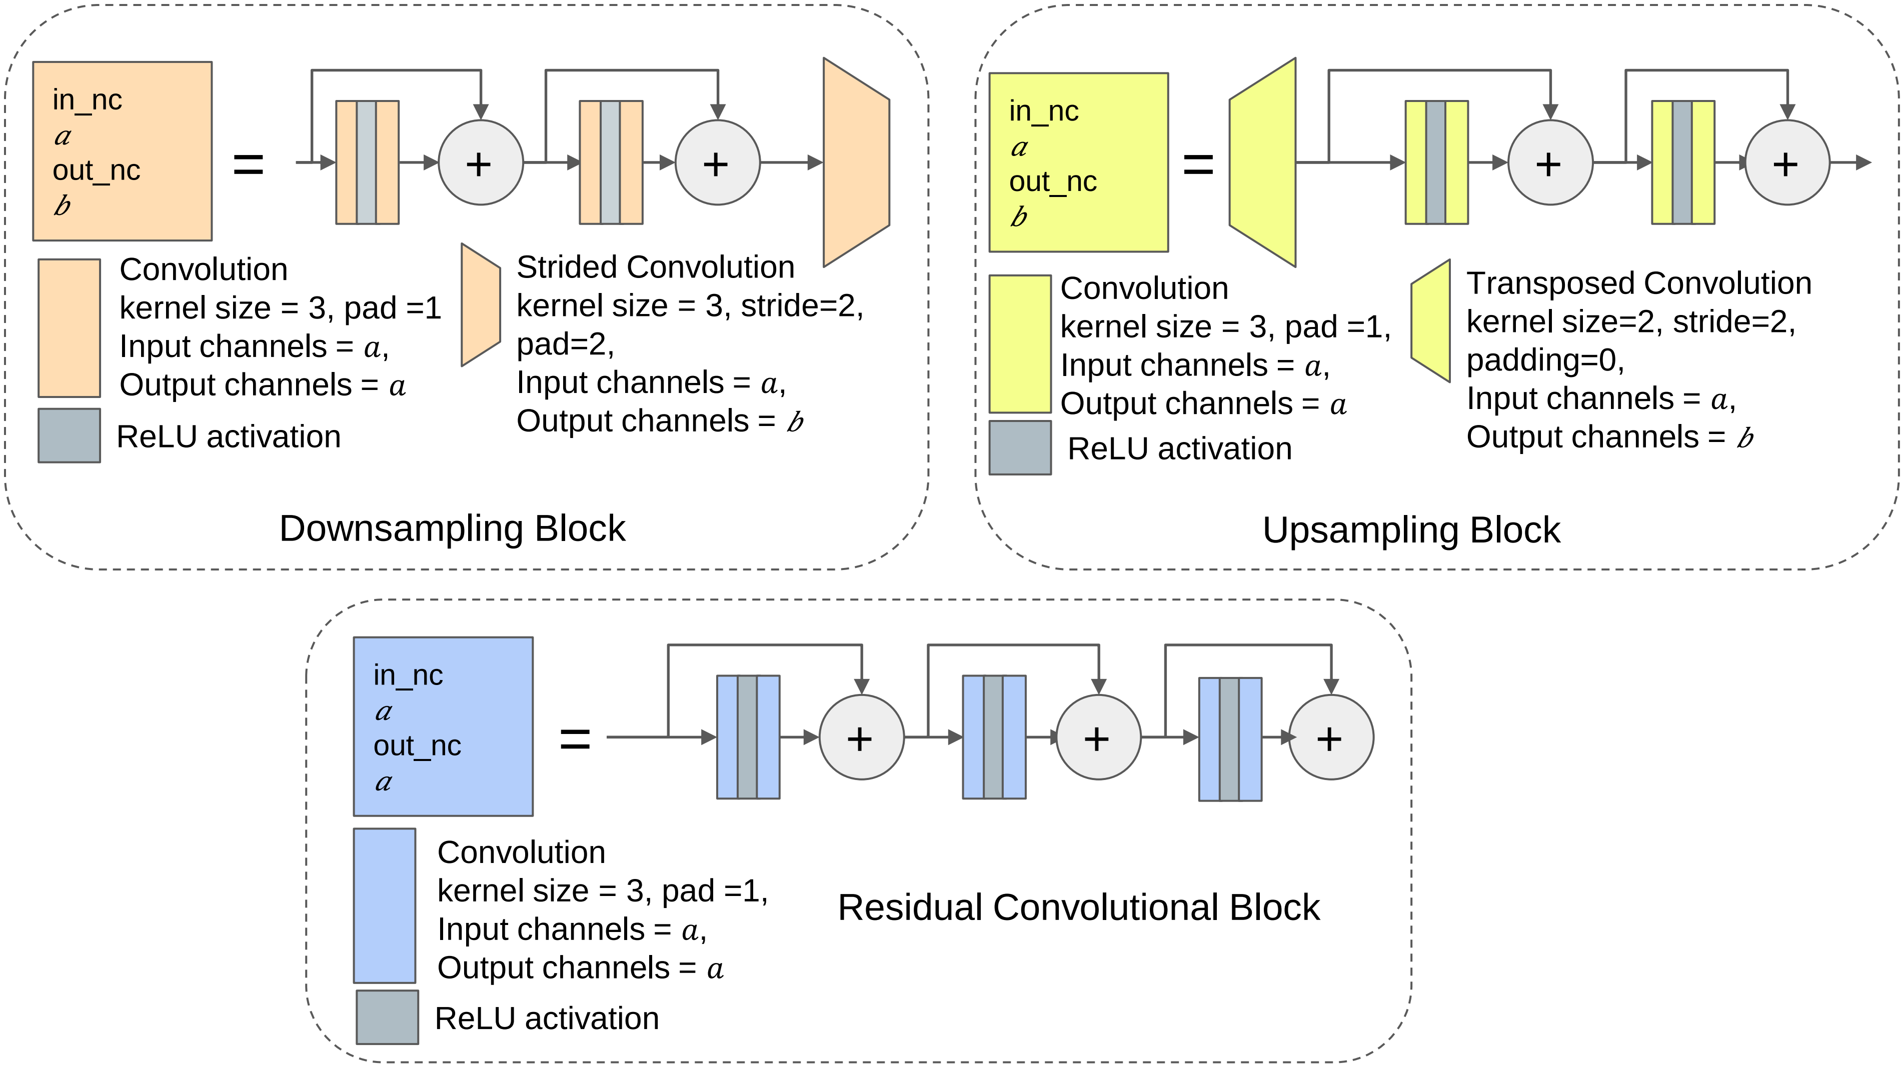
in_nc
a
out_nc
b
=
+
Convolution
kernel size = 3, pad =1
Input channels = a,
Output channels = a
ReLU activation
Strided Convolution
kernel size = 3, stride=2,
pad=2,
Input channels = a,
Output channels = b
Downsampling Block
in_nc
a
out_nc
b
=
+
Convolution
kernel size = 3, pad =1,
Input channels = a,
Output channels = a
ReLU activation
Transposed Convolution
kernel size=2, stride=2,
padding=0,
Input channels = a,
Output channels = b
Upsampling Block
in_nc
a
out_nc
a
=
+
Convolution
kernel size = 3, pad =1,
Input channels = a,
Output channels = a
ReLU activation
Residual Convolutional Block

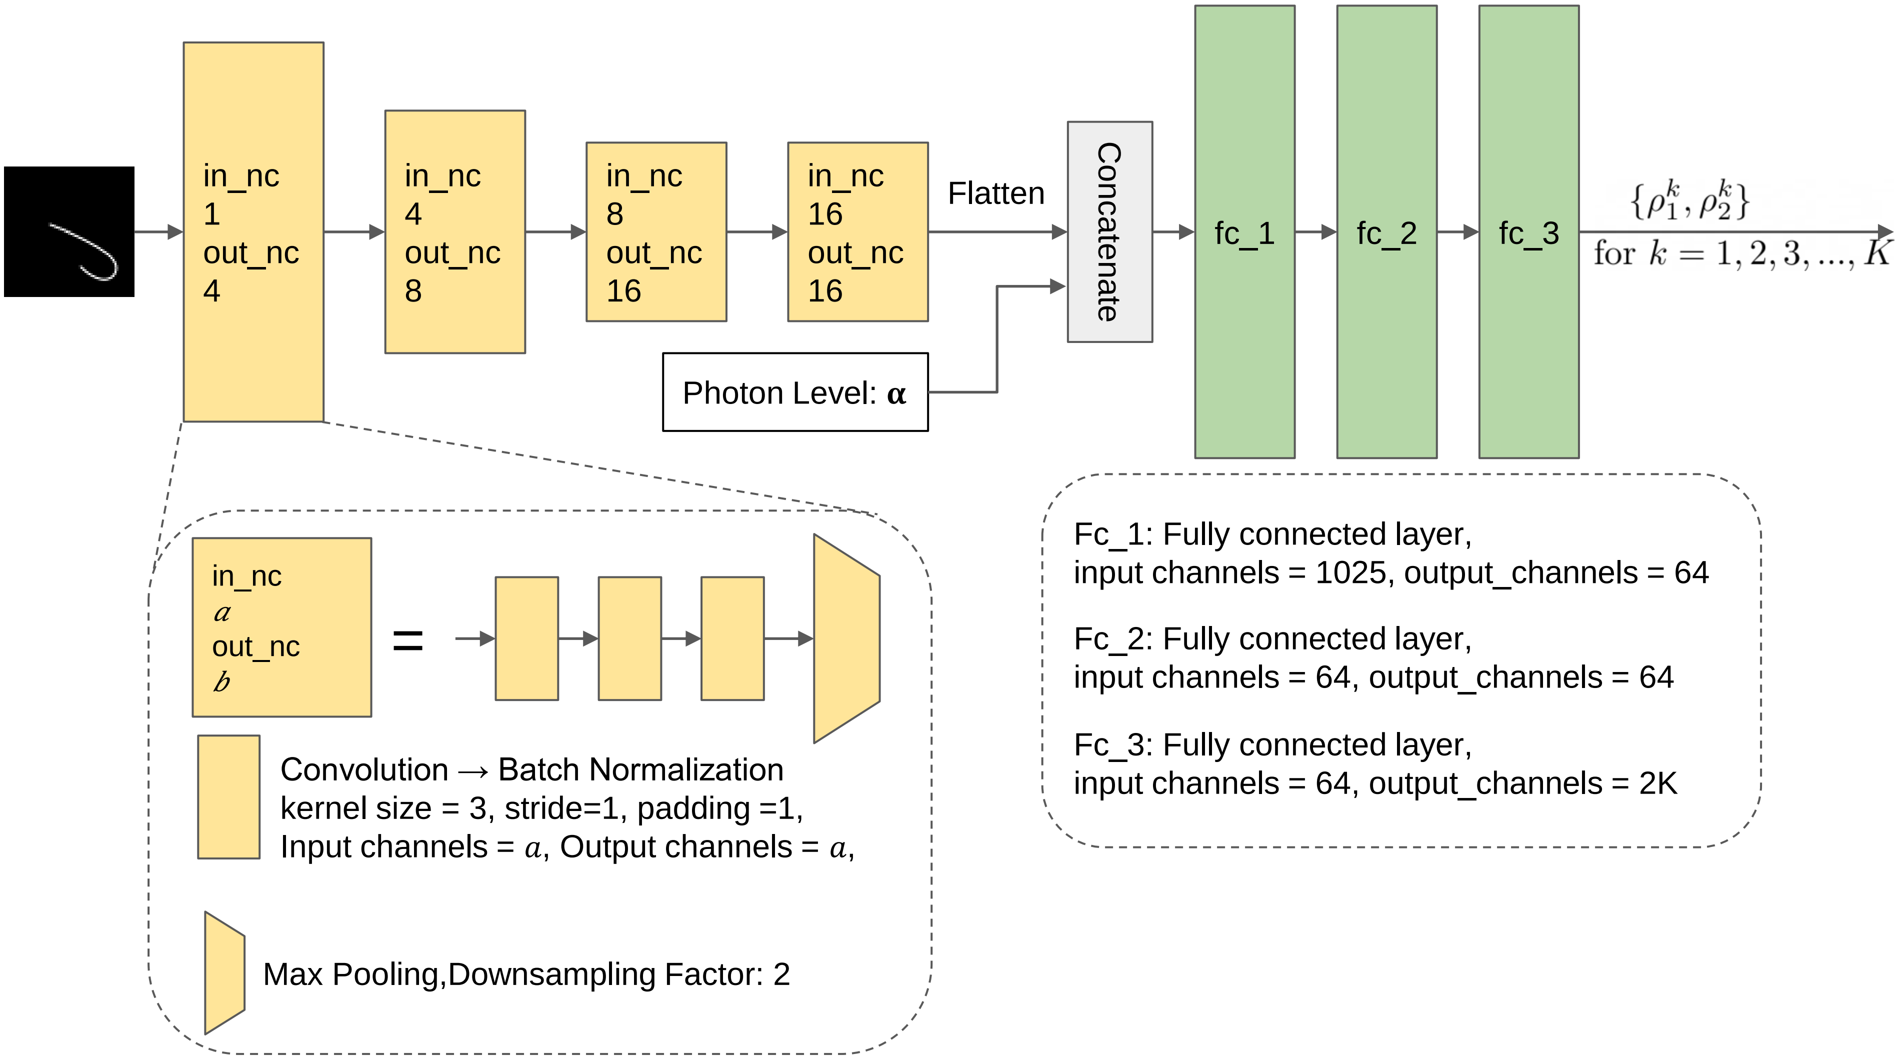
in_nc 1 out_nc 4
in_nc 4 out_nc 8
in_nc 8 out_nc 16
in_nc 16 out_nc 16
Flatten
Concatenate
Photon Level: $\alpha$
fc_1
fc_2
fc_3
$\{\rho_1^k, \rho_2^k\}$
for $k = 1, 2, 3, ..., K$
in_nc $a$ out_nc $b$ =
Convolution → Batch Normalization
kernel size = 3, stride=1, padding =1,
Input channels = $a$, Output channels = $a$,
Max Pooling,Downsampling Factor: 2
Fc_1: Fully connected layer,
input channels = 1025, output_channels = 64
Fc_2: Fully connected layer,
input channels = 64, output_channels = 64
Fc_3: Fully connected layer,
input channels = 64, output_channels = 2K
